# Supplementary material for: Universal Link Predictor By In-Context Learning on Graphs
Source: arXiv:2402.07738 source file (2024-02-15)
Supplement: Supplementary file 1 [file appendix_old.tex]

\begin{table*}[t]
    \centering
    \caption{The pretrain datasets and test benchmarks.}
    \resizebox{\linewidth}{!}{%
    % insert
    \begin{tabular}{lcc|ccccccc}
    \toprule
        \textbf{Dataset} & \textbf{Pretrain} & \textbf{Test} & \textbf{\# Nodes} & \textbf{\# Edges} & \textbf{Avg. node deg.} & \textbf{Std. node deg.} & \textbf{Max. node deg.} & \textbf{Density} & \textbf{Attr. Dimension}\\
    \midrule\rowcolor{Gray}
    \multicolumn{10}{c}{\textbf{Biology}} \\
    Ecoli &\Checkmark & - & 1805 & 29320 & 16.24 & 48.38 & 1030 & 1.8009\% & -\\
    Yeast &\Checkmark & - & 2375 & 23386 & 9.85 & 15.5 & 118 & 0.8295\% & -\\
    Celegans &- & \Checkmark & 297 & 4296 & 14.46 & 12.97 & 134 & 9.7734\% & -\\
    \midrule
    \rowcolor{Gray}
    \multicolumn{10}{c}{\textbf{Transport}} \\
    Power &\Checkmark & - & 4941 & 13188 & 2.67 & 1.79 & 19 & 0.1081\% & -\\
    USAir &- & \Checkmark & 332 & 4252 & 12.81 & 20.13 & 139 & 7.7385\% & -\\
    \midrule
    \rowcolor{Gray}
    \multicolumn{10}{c}{\textbf{Web}} \\
    PolBlogs &\Checkmark & - & 1490 & 19025 & 12.77 & 20.73 & 256 & 1.7150\% & -\\
    Router &\Checkmark & - & 5022 & 12516 & 2.49 & 5.29 & 106 & 0.0993\% & -\\
    PB &- & \Checkmark & 1222 & 33428 & 27.36 & 38.42 & 351 & 4.4808\% & -\\
    \midrule
    \rowcolor{Gray}
    \multicolumn{10}{c}{\textbf{Collaboration}} \\
    Physics &\Checkmark & - & 34493 & 495924 & 14.38 & 15.57 & 382 & 0.0834\% & 8415\\
    CS &- & \Checkmark & 18333 & 163788 & 8.93 & 9.11 & 136 & 0.0975\% & 6805\\
    NS &- & \Checkmark & 1589 & 5484 & 3.45 & 3.47 & 34 & 0.4347\% & -\\
    \midrule
    \rowcolor{Gray}
    \multicolumn{10}{c}{\textbf{Citation}} \\
    Pubmed &\Checkmark & - & 19717 & 88648 & 4.5 & 7.43 & 171 & 0.0456\% & 500\\
    Citeseer &\Checkmark & - & 3327 & 9104 & 2.74 & 3.38 & 99 & 0.1645\% & 3703\\
    Cora &- & \Checkmark & 2708 & 10556 & 3.9 & 5.23 & 168 & 0.2880\% & 1433\\
    \midrule
    \rowcolor{Gray}
    \multicolumn{10}{c}{\textbf{Product}} \\
    Photo &- & \Checkmark & 7650 & 238162 & 31.13 & 47.28 & 1434 & 0.8140\% & 745\\
    \midrule
    \rowcolor{Gray}
    \multicolumn{10}{c}{\textbf{Social}} \\
    Twitch &\Checkmark & - & 34118 & 429113 & 12.58 & 35.88 & 1489 & 0.0737\% & 3170\\
    Github &\Checkmark & - & 37700 & 289003 & 7.67 & 46.59 & 6809 & 0.0407\% & 4005\\
    Facebook &- & \Checkmark & 22470 & 171002 & 7.61 & 15.26 & 472 & 0.0677\% & 4714\\
    \midrule
    \bottomrule
    \end{tabular}
    % until
}
\end{table*}


\begin{table*}[t]
    \centering
    \caption{Link prediction results on benchmarks evaluated by Hits@20.  The format is average score ± standard deviation. The top three models are colored by \textbf{\textcolor{red}{First}}, \textbf{\textcolor{blue}{Second}}, \textbf{\textcolor{violet}{Third}}.}
    \resizebox{\textwidth}{!}{%
    % insert
    \begin{tabular}{lcccccccc}
    \toprule
        & \textbf{Facebook} & \textbf{Cora} & \textbf{USAir} & \textbf{NS} & \textbf{PB} & \textbf{C.ele} & \textbf{CS} & \textbf{Photo}\\\midrule
    \textbf{CN} & $43.35 {\scriptstyle \pm 4.75}$ & \thirdt{33.85}{0.93} & $66.12 {\scriptstyle \pm 2.27}$ & \thirdt{74.03}{1.59} & $27.96 {\scriptstyle \pm 3.58}$ & $28.14 {\scriptstyle \pm 9.17}$ & $38.81 {\scriptstyle \pm 0.38}$ & $22.03 {\scriptstyle \pm 2.61}$ \\
    \textbf{AA} & \thirdt{52.46}{2.95} & $33.85 {\scriptstyle \pm 0.93}$ & \thirdt{76.78}{2.73} & $74.03 {\scriptstyle \pm 1.59}$ & $30.60 {\scriptstyle \pm 3.58}$ & $38.83 {\scriptstyle \pm 6.76}$ & \firstt{57.49}{3.97} & \thirdt{28.65}{3.39} \\
    \textbf{RA} & \firstt{54.60}{2.77} & $33.85 {\scriptstyle \pm 0.93}$ & \firstt{79.76}{3.10} & $74.03 {\scriptstyle \pm 1.59}$ & \thirdt{30.66}{3.42} & \thirdt{40.16}{5.83} & \secondt{56.93}{4.58} & \secondt{29.83}{4.16} \\
    \textbf{PA} & $8.10 {\scriptstyle \pm 0.57}$ & $14.81 {\scriptstyle \pm 1.62}$ & $67.32 {\scriptstyle \pm 3.35}$ & $22.85 {\scriptstyle \pm 4.20}$ & $15.05 {\scriptstyle \pm 2.25}$ & $26.06 {\scriptstyle \pm 4.84}$ & $3.51 {\scriptstyle \pm 0.49}$ & $5.56 {\scriptstyle \pm 0.94}$ \\ \midrule
    \textbf{SEAL} & $48.00 {\scriptstyle \pm 6.35}$ & \firstt{50.19}{5.47} & $74.96 {\scriptstyle \pm 5.72}$ & \firstt{82.61}{2.89} & \secondt{30.90}{2.89} & \secondt{42.10}{5.67} & $50.07 {\scriptstyle \pm 9.35}$ & - \\ \midrule
    \textbf{Ours} & \secondt{54.18}{1.88} & \secondt{47.29}{4.52} & \secondt{79.08}{3.46} & \secondt{80.07}{3.09} & \firstt{31.97}{4.16} & \firstt{44.48}{6.11} & \thirdt{52.01}{5.73} & \firstt{31.39}{4.82} \\
    \bottomrule
    \end{tabular}
    % until
}\vspace{-8pt}
\end{table*}

\begin{table*}[t]
    \centering
    \caption{Link prediction results on benchmarks evaluated by Hits@50.  The format is average score ± standard deviation. The top three models are colored by \textbf{\textcolor{red}{First}}, \textbf{\textcolor{blue}{Second}}, \textbf{\textcolor{violet}{Third}}.}
    \resizebox{\textwidth}{!}{%
    % insert
    \begin{tabular}{lcccccccccc}
    \toprule
        & \textbf{Facebook} & \textbf{Cora} & \textbf{USAir} & \textbf{NS} & \textbf{PB} & \textbf{C.ele} & \textbf{CS} & \textbf{Photo} & \textbf{TRIANGULAR} & \textbf{GRID}\\\midrule
    \textbf{SEAL} & \secondt{64.35}{2.57} & \secondt{59.79}{5.04} & \thirdt{86.02}{4.85} & \secondt{87.48}{2.74} & $47.29 {\scriptstyle \pm 3.32}$ & \firstt{66.15}{3.32} & \firstt{67.44}{6.01} & \firstt{52.52}{4.81} & - & - \\ \midrule
    \textbf{SEAL-Pretrained} & $54.57 {\scriptstyle \pm 1.48}$ & $58.21 {\scriptstyle \pm 2.24}$ & $86.00 {\scriptstyle \pm 1.56}$ & $84.07 {\scriptstyle \pm 1.96}$ & $45.44 {\scriptstyle \pm 2.68}$ & $61.28 {\scriptstyle \pm 3.76}$ & \thirdt{62.82}{1.62} & $35.46 {\scriptstyle \pm 2.04}$ & - & - \\
    \textbf{SEAL-Pretrained+FT} & $57.84 {\scriptstyle \pm 1.66}$ & \firstt{62.19}{3.27} & \firstt{88.49}{2.16} & $84.84 {\scriptstyle \pm 2.32}$ & \thirdt{47.78}{3.32} & \secondt{64.45}{4.14} & $61.54 {\scriptstyle \pm 3.09}$ & $37.29 {\scriptstyle \pm 2.73}$ & \secondt{98.35}{0.57} & \firstt{78.24}{0.79} \\
    \textbf{SEAL-ICL} & \firstt{65.37}{2.12} & $53.10 {\scriptstyle \pm 3.23}$ & $75.39 {\scriptstyle \pm 7.82}$ & \thirdt{85.89}{3.31} & \firstt{48.46}{3.17} & $64.34 {\scriptstyle \pm 4.52}$ & $58.60 {\scriptstyle \pm 11.17}$ & $28.23 {\scriptstyle \pm 3.36}$ & \firstt{98.73}{0.54} & $51.64 {\scriptstyle \pm 14.52}$ \\ \midrule
    \textbf{MPLP} & $64.07 {\scriptstyle \pm 2.41}$ & \thirdt{59.21}{1.90} & $81.65 {\scriptstyle \pm 4.81}$ & \firstt{89.23}{1.61} & \secondt{48.17}{3.11} & \thirdt{64.45}{3.79} & \secondt{64.19}{2.76} & \secondt{49.06}{3.43} & - & - \\
    \textbf{MPLP-Pretrained} & $56.77 {\scriptstyle \pm 2.06}$ & $56.77 {\scriptstyle \pm 2.23}$ & \secondt{86.35}{1.85} & $80.57 {\scriptstyle \pm 1.43}$ & $44.55 {\scriptstyle \pm 1.83}$ & $61.17 {\scriptstyle \pm 5.08}$ & $44.46 {\scriptstyle \pm 0.97}$ & $43.30 {\scriptstyle \pm 3.60}$ & $87.33 {\scriptstyle \pm 0.88}$ & \thirdt{55.87}{1.00} \\
    \textbf{MPLP-ICL} & \thirdt{64.14}{1.80} & $56.56 {\scriptstyle \pm 2.00}$ & $84.14 {\scriptstyle \pm 2.85}$ & $79.85 {\scriptstyle \pm 1.51}$ & $43.42 {\scriptstyle \pm 1.70}$ & $60.51 {\scriptstyle \pm 3.55}$ & $52.36 {\scriptstyle \pm 1.15}$ & \thirdt{43.63}{3.70} & \thirdt{88.81}{0.69} & \secondt{56.20}{1.05} \\
    \bottomrule
    \end{tabular}
    % until
}\vspace{-8pt}
\end{table*}


\begin{table*}[t]
    \centering
    \caption{Link prediction results on benchmarks evaluated by Hits@50.  The format is average score ± standard deviation. The top three models are colored by \textbf{\textcolor{red}{First}}, \textbf{\textcolor{blue}{Second}}, \textbf{\textcolor{violet}{Third}}.}
    \resizebox{\textwidth}{!}{%
    % insert
    \begin{tabular}{lccccccccc}
    \toprule
    % \rowcolor{Gray}
            &\multicolumn{1}{c}{Biology}&\multicolumn{1}{c}{Transport}&\multicolumn{1}{c}{Web}&\multicolumn{2}{c}{Collaboration}&\multicolumn{1}{c}{Citation}&\multicolumn{1}{c}{Social}&\multicolumn{1}{c}{Product}\\ \cmidrule(r{0.5em}){2-2} \cmidrule(r{0.5em}){3-3} \cmidrule(r{0.5em}){4-4} \cmidrule(r{0.5em}){5-6} \cmidrule(r{0.5em}){7-7} \cmidrule(r{0.5em}){8-8}  \cmidrule(r{0.5em}){9-9} 
            
        & \textbf{C.ele} & \textbf{USAir} & \textbf{PB} & \textbf{NS} & \textbf{CS} & \textbf{Cora} & \textbf{Facebook} & \textbf{Photo}\\\midrule
    \textbf{CN} & $46.88 {\scriptstyle \pm 12.28}$ & $82.75 {\scriptstyle \pm 1.54}$ & $41.15 {\scriptstyle \pm 3.77}$ & $74.03 {\scriptstyle \pm 1.59}$ & $56.84 {\scriptstyle \pm 15.56}$ & $33.85 {\scriptstyle \pm 0.93}$ & $58.70 {\scriptstyle \pm 0.35}$ & $32.40 {\scriptstyle \pm 2.66}$ & 53.32 \\
    \textbf{AA} & $61.07 {\scriptstyle \pm 5.16}$ & $86.96 {\scriptstyle \pm 2.24}$ & $44.12 {\scriptstyle \pm 3.36}$ & $74.03 {\scriptstyle \pm 1.59}$ & \firstt{68.22}{1.08} & $33.85 {\scriptstyle \pm 0.93}$ & \secondt{67.80}{2.12} & \secondt{41.26}{3.39} & 59.66 \\
    \textbf{RA} & $62.80 {\scriptstyle \pm 4.84}$ & \thirdt{87.27}{1.89} & $43.72 {\scriptstyle \pm 2.86}$ & $74.03 {\scriptstyle \pm 1.59}$ & \secondt{68.21}{1.08} & $33.85 {\scriptstyle \pm 0.93}$ & \firstt{68.84}{2.03} & \firstt{46.08}{3.34} & 60.60 \\
    \textbf{PA} & $43.85 {\scriptstyle \pm 4.12}$ & $77.69 {\scriptstyle \pm 2.29}$ & $28.93 {\scriptstyle \pm 1.91}$ & $35.35 {\scriptstyle \pm 3.01}$ & $6.49 {\scriptstyle \pm 0.61}$ & $22.09 {\scriptstyle \pm 1.52}$ & $12.95 {\scriptstyle \pm 0.63}$ & $9.24 {\scriptstyle \pm 1.11}$ & 29.57 \\ \midrule
    \textbf{SP} & $0.00 {\scriptstyle \pm 0.00}$ & $0.00 {\scriptstyle \pm 0.00}$ & $0.00 {\scriptstyle \pm 0.00}$ & $80.00 {\scriptstyle \pm 1.11}$ & $41.34 {\scriptstyle \pm 35.58}$ & $52.97 {\scriptstyle \pm 1.53}$ & $0.00 {\scriptstyle \pm 0.00}$ & $0.00 {\scriptstyle \pm 0.00}$ & 21.79 \\
    \textbf{Katz} & $58.86 {\scriptstyle \pm 6.48}$ & $84.64 {\scriptstyle \pm 1.86}$ & $44.36 {\scriptstyle \pm 3.65}$ & $78.96 {\scriptstyle \pm 1.35}$ & \thirdt{66.32}{5.59} & $52.97 {\scriptstyle \pm 1.53}$ & $60.79 {\scriptstyle \pm 0.60}$ & $34.01 {\scriptstyle \pm 3.41}$ & 60.11 \\
    \textbf{SEAL} & \firstt{67.06}{4.19} & \secondt{87.93}{4.08} & \thirdt{47.98}{3.65} & \secondt{88.36}{1.08} & $64.47 {\scriptstyle \pm 2.66}$ & \firstt{63.70}{2.59} & $65.15 {\scriptstyle \pm 4.55}$ & \thirdt{40.55}{5.16} & 65.65 \\ \midrule
    \textbf{SEAL-Pretrained} & $61.28 {\scriptstyle \pm 3.76}$ & $86.00 {\scriptstyle \pm 1.56}$ & $45.44 {\scriptstyle \pm 2.68}$ & $84.07 {\scriptstyle \pm 1.96}$ & $62.82 {\scriptstyle \pm 1.62}$ & \thirdt{58.21}{2.24} & $54.57 {\scriptstyle \pm 1.48}$ & $35.46 {\scriptstyle \pm 2.04}$ & 60.98 \\
    \textbf{SEAL-Pretrained+FT} & $64.45 {\scriptstyle \pm 4.14}$ & \firstt{88.49}{2.16} & $47.78 {\scriptstyle \pm 3.32}$ & $84.84 {\scriptstyle \pm 2.32}$ & $61.54 {\scriptstyle \pm 3.09}$ & \secondt{62.19}{3.27} & $58.70 {\scriptstyle \pm 2.78}$ & $37.74 {\scriptstyle \pm 3.15}$ & 63.22 \\
    \textbf{SEAL-ICL-100} & \thirdt{64.97}{4.32} & $80.87 {\scriptstyle \pm 4.49}$ & \firstt{48.52}{2.99} & \thirdt{88.01}{2.46} & $63.93 {\scriptstyle \pm 3.53}$ & $55.86 {\scriptstyle \pm 3.31}$ & $65.45 {\scriptstyle \pm 2.11}$ & $29.19 {\scriptstyle \pm 4.86}$ & 62.10 \\
    \textbf{SEAL-ICL-200} & \secondt{65.20}{4.40} & $85.98 {\scriptstyle \pm 2.00}$ & \secondt{48.14}{2.99} & \firstt{89.09}{2.05} & $64.59 {\scriptstyle \pm 2.65}$ & $57.50 {\scriptstyle \pm 2.40}$ & \thirdt{65.49}{2.05} & $34.83 {\scriptstyle \pm 3.24}$ & 63.85 \\
    \bottomrule
    \end{tabular}
    % until
}\vspace{-8pt}
\end{table*}


\begin{table*}[t]
    \centering
    \caption{Link prediction results on benchmarks evaluated by Hits@100.  The format is average score ± standard deviation. The top three models are colored by \textbf{\textcolor{red}{First}}, \textbf{\textcolor{blue}{Second}}, \textbf{\textcolor{violet}{Third}}.}
    \resizebox{\textwidth}{!}{%
    % insert
    \begin{tabular}{lcccccccc}
    \toprule
        & \textbf{Facebook} & \textbf{Cora} & \textbf{USAir} & \textbf{NS} & \textbf{PB} & \textbf{C.ele} & \textbf{CS} & \textbf{Photo}\\\midrule
    \textbf{CN} & $68.20 {\scriptstyle \pm 0.24}$ & \thirdt{33.85}{0.93} & $85.74 {\scriptstyle \pm 4.37}$ & \thirdt{74.03}{1.59} & $53.49 {\scriptstyle \pm 0.68}$ & $57.41 {\scriptstyle \pm 2.75}$ & \secondt{68.80}{0.38} & $43.91 {\scriptstyle \pm 2.79}$ \\
    \textbf{AA} & \secondt{75.51}{1.00} & $33.85 {\scriptstyle \pm 0.93}$ & \thirdt{92.00}{0.99} & $74.03 {\scriptstyle \pm 1.59}$ & \thirdt{57.16}{1.84} & $76.39 {\scriptstyle \pm 3.54}$ & \thirdt{68.80}{0.38} & \secondt{53.64}{3.15} \\
    \textbf{RA} & \firstt{76.05}{0.90} & $33.85 {\scriptstyle \pm 0.93}$ & $92.00 {\scriptstyle \pm 0.99}$ & $74.03 {\scriptstyle \pm 1.59}$ & $56.94 {\scriptstyle \pm 1.75}$ & \thirdt{76.53}{3.28} & $68.80 {\scriptstyle \pm 0.38}$ & \firstt{59.26}{1.79} \\
    \textbf{PA} & $18.14 {\scriptstyle \pm 0.66}$ & $30.73 {\scriptstyle \pm 1.64}$ & $84.78 {\scriptstyle \pm 1.47}$ & $44.89 {\scriptstyle \pm 3.72}$ & $43.72 {\scriptstyle \pm 2.22}$ & $57.46 {\scriptstyle \pm 3.00}$ & $9.96 {\scriptstyle \pm 0.59}$ & $14.17 {\scriptstyle \pm 0.67}$ \\ \midrule
    \textbf{SEAL} & \thirdt{75.46}{2.06} & \firstt{68.33}{3.99} & \secondt{94.45}{2.86} & \firstt{92.46}{1.41} & \firstt{60.64}{3.43} & \firstt{82.52}{1.81} & \firstt{76.16}{2.84} & - \\ \midrule
    \textbf{Ours} & $64.36 {\scriptstyle \pm 2.86}$ & \secondt{55.79}{6.46} & \firstt{94.52}{1.26} & \secondt{85.53}{4.40} & \secondt{59.54}{1.70} & \secondt{80.05}{3.07} & $68.19 {\scriptstyle \pm 3.82}$ & \thirdt{47.87}{6.99} \\
    \bottomrule
    \end{tabular}
    % until
}\vspace{-8pt}
\end{table*}


\begin{table*}[t]
    \centering
    \caption{Link prediction results on benchmarks evaluated by AUCROC.  The format is average score ± standard deviation. The top three models are colored by \textbf{\textcolor{red}{First}}, \textbf{\textcolor{blue}{Second}}, \textbf{\textcolor{violet}{Third}}.}
    \resizebox{\textwidth}{!}{%
    % insert
    \begin{tabular}{lcccccccc}
    \toprule
        & \textbf{Facebook} & \textbf{Cora} & \textbf{USAir} & \textbf{NS} & \textbf{PB} & \textbf{C.ele} & \textbf{CS} & \textbf{Photo}\\\midrule
    \textbf{CN} & $90.14 {\scriptstyle \pm 0.10}$ & $66.70 {\scriptstyle \pm 0.49}$ & $92.24 {\scriptstyle \pm 0.79}$ & $86.96 {\scriptstyle \pm 0.78}$ & $90.15 {\scriptstyle \pm 0.32}$ & $79.84 {\scriptstyle \pm 2.05}$ & $84.30 {\scriptstyle \pm 0.19}$ & $95.35 {\scriptstyle \pm 0.11}$ \\
    \textbf{AA} & \thirdt{90.18}{0.10} & \thirdt{66.74}{0.49} & $93.15 {\scriptstyle \pm 0.78}$ & $86.98 {\scriptstyle \pm 0.79}$ & $90.49 {\scriptstyle \pm 0.31}$ & $81.44 {\scriptstyle \pm 1.93}$ & \thirdt{84.32}{0.19} & \secondt{95.63}{0.09} \\
    \textbf{RA} & $90.18 {\scriptstyle \pm 0.10}$ & $66.74 {\scriptstyle \pm 0.49}$ & \thirdt{93.44}{0.76} & \thirdt{86.99}{0.79} & \thirdt{90.53}{0.27} & \thirdt{81.68}{1.81} & $84.32 {\scriptstyle \pm 0.19}$ & \firstt{95.77}{0.09} \\
    \textbf{PA} & $85.05 {\scriptstyle \pm 0.15}$ & $63.52 {\scriptstyle \pm 1.26}$ & $88.72 {\scriptstyle \pm 0.97}$ & $67.55 {\scriptstyle \pm 1.47}$ & $89.77 {\scriptstyle \pm 0.22}$ & $74.25 {\scriptstyle \pm 1.93}$ & $73.80 {\scriptstyle \pm 0.24}$ & $83.23 {\scriptstyle \pm 0.20}$ \\ \midrule
    \textbf{SEAL} & \firstt{98.16}{0.17} & \firstt{86.81}{1.63} & \secondt{94.93}{1.40} & \firstt{95.78}{0.74} & \firstt{94.22}{0.33} & \firstt{87.19}{0.73} & \firstt{96.49}{0.31} & - \\ \midrule
    \textbf{Ours} & \secondt{93.67}{1.39} & \secondt{86.19}{1.35} & \firstt{95.48}{0.65} & \secondt{94.46}{1.28} & \secondt{92.50}{0.69} & \secondt{86.27}{1.68} & \secondt{93.63}{0.75} & \thirdt{95.38}{1.21} \\
    \bottomrule
    \end{tabular}
    % until
}\vspace{-8pt}
\end{table*}

\begin{table*}[t]
    \centering
    \caption{Link prediction results on benchmarks evaluated by AUCPR.  The format is average score ± standard deviation. The top three models are colored by \textbf{\textcolor{red}{First}}, \textbf{\textcolor{blue}{Second}}, \textbf{\textcolor{violet}{Third}}.}
    \resizebox{\textwidth}{!}{%
    % insert
    \begin{tabular}{lcccccccc}
    \toprule
        & \textbf{Facebook} & \textbf{Cora} & \textbf{USAir} & \textbf{NS} & \textbf{PB} & \textbf{C.ele} & \textbf{CS} & \textbf{Photo}\\\midrule
    \textbf{CN} & $94.92 {\scriptstyle \pm 0.05}$ & $82.77 {\scriptstyle \pm 0.43}$ & $93.84 {\scriptstyle \pm 0.65}$ & $93.43 {\scriptstyle \pm 0.38}$ & $91.65 {\scriptstyle \pm 0.41}$ & $81.41 {\scriptstyle \pm 2.44}$ & $92.04 {\scriptstyle \pm 0.10}$ & \thirdt{96.69}{0.08} \\
    \textbf{AA} & $94.97 {\scriptstyle \pm 0.05}$ & \thirdt{82.89}{0.40} & $94.77 {\scriptstyle \pm 0.63}$ & $93.46 {\scriptstyle \pm 0.39}$ & \thirdt{91.95}{0.40} & $83.01 {\scriptstyle \pm 2.24}$ & \thirdt{92.07}{0.11} & \secondt{97.08}{0.07} \\
    \textbf{RA} & \thirdt{94.98}{0.05} & $82.88 {\scriptstyle \pm 0.40}$ & \thirdt{95.14}{0.62} & \thirdt{93.47}{0.39} & $91.93 {\scriptstyle \pm 0.37}$ & \thirdt{83.40}{1.95} & $92.06 {\scriptstyle \pm 0.11}$ & \firstt{97.26}{0.06} \\
    \textbf{PA} & $87.04 {\scriptstyle \pm 0.09}$ & $68.54 {\scriptstyle \pm 1.34}$ & $91.19 {\scriptstyle \pm 0.74}$ & $71.60 {\scriptstyle \pm 1.87}$ & $89.25 {\scriptstyle \pm 0.36}$ & $74.90 {\scriptstyle \pm 2.69}$ & $75.94 {\scriptstyle \pm 0.23}$ & $83.87 {\scriptstyle \pm 0.21}$ \\ \midrule
    \textbf{SEAL} & \firstt{98.47}{0.15} & \firstt{89.27}{1.39} & \secondt{95.23}{1.25} & \firstt{96.74}{0.52} & \firstt{93.97}{0.46} & \firstt{86.43}{1.24} & \firstt{97.19}{0.27} & - \\ \midrule
    \textbf{Ours} & \secondt{95.03}{0.99} & \secondt{87.97}{1.49} & \firstt{95.54}{0.72} & \secondt{95.53}{1.02} & \secondt{92.47}{0.61} & \secondt{86.15}{2.36} & \secondt{95.07}{0.56} & $95.91 {\scriptstyle \pm 1.04}$ \\
    \bottomrule
    \end{tabular}
    % until
}\vspace{-8pt}
\end{table*}


\begin{table*}[t]
    \centering
    \caption{Link prediction results on benchmarks evaluated by AUCROC.  The format is average score ± standard deviation. The top three models are colored by \textbf{\textcolor{red}{First}}, \textbf{\textcolor{blue}{Second}}, \textbf{\textcolor{violet}{Third}}.}
    \resizebox{\textwidth}{!}{%
    % insert
    \begin{tabular}{lcc}
    \toprule
        & \textbf{TRIANGULAR} & \textbf{GRID}\\\midrule
    \textbf{CN} & $86.73 {\scriptstyle \pm 0.41}$ & $49.96 {\scriptstyle \pm 0.01}$ \\
    \textbf{AA} & $86.73 {\scriptstyle \pm 0.42}$ & $49.96 {\scriptstyle \pm 0.01}$ \\
    \textbf{RA} & $86.72 {\scriptstyle \pm 0.42}$ & $49.96 {\scriptstyle \pm 0.01}$ \\
    \textbf{PA} & $29.34 {\scriptstyle \pm 0.58}$ & $23.92 {\scriptstyle \pm 0.66}$ \\ \midrule
    \textbf{SEAL(40)} & \secondt{99.59}{0.12} & \secondt{96.93}{0.85} \\
    \textbf{SEAL} & \firstt{99.91}{0.04} & \firstt{98.11}{0.10} \\ \midrule
    \textbf{Ours} & \thirdt{99.32}{0.45} & \thirdt{96.52}{0.32} \\
    \bottomrule
    \end{tabular}
    % until
}\vspace{-8pt}
\end{table*}
\begin{table*}[t]
    \centering
    \caption{Link prediction results on benchmarks evaluated by AUCPR.  The format is average score ± standard deviation. The top three models are colored by \textbf{\textcolor{red}{First}}, \textbf{\textcolor{blue}{Second}}, \textbf{\textcolor{violet}{Third}}.}
    \resizebox{\textwidth}{!}{%
    % insert
    \begin{tabular}{lcc}
    \toprule
        & \textbf{TRIANGULAR} & \textbf{GRID}\\\midrule
    \textbf{CN} & $93.29 {\scriptstyle \pm 0.22}$ & $25.00 {\scriptstyle \pm 0.00}$ \\
    \textbf{AA} & $93.26 {\scriptstyle \pm 0.24}$ & $25.00 {\scriptstyle \pm 0.00}$ \\
    \textbf{RA} & $93.26 {\scriptstyle \pm 0.24}$ & $25.00 {\scriptstyle \pm 0.00}$ \\
    \textbf{PA} & $36.73 {\scriptstyle \pm 0.21}$ & $34.48 {\scriptstyle \pm 0.15}$ \\ \midrule
    \textbf{SEAL(40)} & \thirdt{99.34}{0.21} & \secondt{97.44}{0.44} \\
    \textbf{SEAL} & \firstt{99.89}{0.05} & \firstt{98.23}{0.09} \\ \midrule
    \textbf{Ours} & \secondt{99.45}{0.23} & \thirdt{96.42}{0.18} \\
    \bottomrule
    \end{tabular}
    % until
}\vspace{-8pt}
\end{table*}

\begin{table*}[t]
    \centering
    \caption{Link prediction results on benchmarks evaluated by Hits@100.  The format is average score ± standard deviation. The top three models are colored by \textbf{\textcolor{red}{First}}, \textbf{\textcolor{blue}{Second}}, \textbf{\textcolor{violet}{Third}}.}
    \resizebox{\textwidth}{!}{%
    % insert
    \begin{tabular}{lcc}
    \toprule
        & \textbf{TRIANGULAR} & \textbf{GRID}\\\midrule
    \textbf{CN} & $73.58 {\scriptstyle \pm 0.81}$ & $0.00 {\scriptstyle \pm 0.00}$ \\
    \textbf{AA} & $73.58 {\scriptstyle \pm 0.81}$ & $0.00 {\scriptstyle \pm 0.00}$ \\
    \textbf{RA} & $73.58 {\scriptstyle \pm 0.81}$ & $0.00 {\scriptstyle \pm 0.00}$ \\
    \textbf{PA} & $0.00 {\scriptstyle \pm 0.00}$ & $0.00 {\scriptstyle \pm 0.00}$ \\ \midrule
    \textbf{SEAL(40)} & \secondt{99.55}{0.18} & \secondt{81.08}{1.81} \\
    \textbf{SEAL} & \firstt{99.71}{0.09} & \firstt{83.08}{0.89} \\ \midrule
    \textbf{Ours} & \thirdt{98.79}{0.41} & \thirdt{79.53}{4.81} \\
    \bottomrule
    \end{tabular}
    % until
}\vspace{-8pt}
\end{table*}
